# Supplementary material for: S-PLUS Clusters And Large-scale Environments (SCALE): I. A catalog of known clusters and groups in DR5 and a pilot study of Abell 4038
Source: arXiv:2607.02704 source file (2026-07-02)
Supplement: Supplementary file 1 [file Supplementary_Tables.tex]

\appendix

\section{Supplementary tables} \label{sec:sup-tables}

This section presents Tables 2a and 2b, the supplementary tables referenced in this work. Table \ref{tab:column_description} describes the columns used in Table \ref{tab:compilation}, which lists the spectroscopic members and interlopers for all clusters in Table \ref{tab:59clusters}, as defined in Section \ref{sec:Sample}.

\begin{center}
\startlongtable
\begin{deluxetable*}{rp{0.75\linewidth}}
\tablecaption{%
Description of the columns in Table \ref{tab:compilation}, \ref{tab:a168}, listed in their order of appearance. Column names marked with an asterisk (*) denote patterns representing multiple columns. Table \ref{tab:compilation} includes an additional leading column with the cluster ID, while Table \ref{tab:a168} includes an extra column, flag_member_phot, indicating photometric membership status (0 = member; 1 = interloper; –1 = not considered; see Section \ref{sec:Elismar-Section}).
\label{tab:column_description}
}
\tablehead{%
\colhead{Column name} & \colhead{Description}
}
\startdata
*RA and Dec & right ascension and declination, epoch 2000, in degrees, 2 columns {\bf from here on - from S-PLUS DR5)}\\
PROB\_GAL & Probability of the object of being a galaxy, according to Nakazono et al. (XX)\\
*A and B & profile RMS along the major and minor axis, in degrees (2 columns) \\
THETA & position angle (CCW/World-x), in degrees\\
ELLIPTICITY & A\_IMAGE/B\_IMAGE\\
PETRO\_RADIUS & petrosian apertures in units of A or B\\
*FLUX\_RADIUS\_20/50/90 & radius enclosing 20\%, 50\% or 90\% of the total flux (3 columns) \\
*MU\_MAX\_\texttt{BAND} &  instrumental Peak surface brightness above background in \texttt{BAND}, where \texttt{BAND} is one of: g, r; e.g. MU\_MAX\_g (2 columns) \\
*BACKGROUND\_\texttt{BAND} & instrumental background at centroid position in  \texttt{BAND}, where \texttt{BAND} is one of: g, r; e.g. BACKGROUND\_r (2 columns) \\
*s2n\_\texttt{BAND}\_auto & signal to noise ratio of \texttt{BAND} measurement, where \texttt{BAND} is one of: g, r; e.g. s2n\_g\_auto (2 columns) \\
*\texttt{BAND}\_\texttt{APER} & S-PLUS DR5 AB-calibrated magnitude for the  \texttt{BAND} with aperture \texttt{APER}, where \texttt{BAND} is one of: J0378, J0395, J0410, J0430, J0515, J0660, J0861, g, i, r, u, z, and \texttt{APER} is one of: auto and PStotal; e.g. J0861\_PStotal. (24 columns) \\
*e\_\texttt{BAND}\_\texttt{APER} & S-PLUS DR5 magnitude error for the  \texttt{BAND} with aperture \texttt{APER}, where \texttt{BAND} is one of: J0378, J0395, J0410, J0430, J0515, J0660, J0861, g, i, r, u, z, and \texttt{APER} is one of: auto, PStotal, aper6; e.g. e\_r\_auto. (36 columns) \\
*\texttt{BAND}\_\texttt{APER} & extra S-PLUS DR5 AB-calibrated magnitude for the  \texttt{BAND} with aperture \texttt{APER}, where \texttt{BAND} is one of: g, r and \texttt{APER} is one of: aper3, aper6, res, iso, petro; e.g. r\_petro (10 columns) \\
zml & the single-point estimate of the photometric redshift\\
odds & area of the PDF contained within an interval of 0.02 of the PDF peak\\
*pdf\_weights\_\texttt{i} & weights of the gaussian components of the PDF mixture of the photometric redshift, where \texttt{i} is one of: 0, 1, 2; e.g. pdf\_weights\_0 (3 columns) \\
*pdf\_means\_\texttt{i} & means of the gaussian components of the PDF mixture of the photometric redshift, where \texttt{i} is one of: 0, 1, 2; e.g. pdf\_stds\_1 (3 columns) \\
*pdf\_stds\_\texttt{i} & standard deviations of the gaussian components of the PDF mixture of the photometric redshift, where \texttt{i} is one of: 0, 1, 2; e.g. pdf\_means\_2 (3 columns) \\
radius\_deg & distance to the cluster center, in degrees {\bf (from here on - derived in this work)}\\
radius\_Mpc & distance to the cluster center, in Mpc\\
flag\_member & indication if the object is an spectroscopic member or not of the cluster/group. 0 = member; 1 = interloper; -1 = not considered, following Section \ref{sec:Sample} \\
v & velocity, in km/s\\
v\_err & velocity error, in km/s\\
v\_offset & relative to the cluster central velocity, in km/s\\
z & spectroscopic redshift {\bf (from here on - taken from the compilation of Lima et al. 2025)} \\
e\_z & error in the spectroscopic redshift\\
f\_z & flag for the spectroscopic redshift quality\\
class\_spec & spectroscopic classification of the object\\
original\_class\_spec & original spectroscopic classification of the object (before grouping)\\
source & catalogue from which the the spectroscopic redshift was obtained\\
*mag\_\texttt{BAND} & Legacy Survey DR10 magnitude for band \texttt{BAND}, where \texttt{BAND} is one of: g, r, i, z, w1, w2, w3, w4; e.g: mag\_r (8 columns, {\bf from here on - taken from Tractor table of the Legacy Survey}) \\
type & Legacy Survey DR10 morphological classification, \\
shape\_r & Legacy Survey DR10 effective radius - radius that contains 50\% of the light, in arcsec, see more information in \url{https://www.legacysurvey.org/dr10/description/#morphological-classification}\\
\enddata
\end{deluxetable*}
\end{center}

% RC - Here we include the section 3.3 which was removed from the main body of the paper, with the description of the tables and interlopers in the 58 clusters/groups and the additional data for Abell 168 and MKW4. Cleaning all previous comments.

\subsection{Members and interlopers in 83 cluster/groups} 
\label{sec:membership-tables}

This section describes Table \ref{tab:compilation}. Its columns are detailed in Table \ref{tab:column_description} (see Section \ref{sec:sup-tables}), with two additions: (1) cluster$\_$name, included at the beginning of Table \ref{tab:compilation} to identify the host cluster/group, and (2) flag$\_$member$\_$photoz, appended to Tables \ref{tab:a168} and \ref{tab:mkw4} to indicate photometric membership, as defined in Section \ref{sec:Elismar-Section}.

Table \ref{tab:compilation} lists spec-z’s from the compilation of \citet{Lima+24}, photo-z’s from S-PLUS DR5, and additional parameters for galaxies within $5 \times R_{200}$ of the 83 clusters/groups, classified as spectroscopic members or interlopers using the shifting-gapper technique (Section \ref{sec:Sample}).

\begin{center}
\startlongtable
\tabletypesize{\small} % Reduz tamanho da fonte
\setlength{\tabcolsep}{2.5pt} % Reduz espaçamento entre colunas
\begin{deluxetable*}{*{15}{c}}
\tablecaption{
Spectroscopic members and interlopers for 83 clusters and groups\label{tab:compilation}
}
\tablehead{\colhead{Cluster ID} &
\colhead{RA} & \colhead{Dec} & \colhead{$\cdots$} & \colhead{r\_aper} & \colhead{g\_aper} & \colhead{$\cdots$} & \colhead{zml} & \colhead{odds} & \colhead{$\cdots$} & \colhead{v} & \colhead{v\_err} & \colhead{radius\_deg} & \colhead{radius\_Mpc} & \colhead{v\_offset}
}

\startdata
MKW4 & 180.975 &  1.891  & $\cdots$ & ------  & ------  & $\cdots$ &  ------ & ------  & $\cdots$ & 7325.729  & 3.297 & 0.014 & 0.021 & 1303.803  \\
MKW4 & 181.024 &  1.846  & $\cdots$ & 14.932  & 15.796  & $\cdots$ & 0.023   & 0.999  & $\cdots$ & 4909.101  & 2.098 & 0.053 & 0.079 & -1065.439   \\
MKW4 & 180.966 &  1.836  & $\cdots$ & ------  & ------  & $\cdots$ & ------  & ------ & $\cdots$ & 5686.763  & 9.293 & 0.057 & 0.084 & -303.026   \\
$\cdots$ & $\cdots$ & $\cdots$ & $\cdots$ & $\cdots$ & $\cdots$ & $\cdots$ & $\cdots$ & $\cdots$ & $\cdots$ & $\cdots$ & $\cdots$ & $\cdots$ & $\cdots$ & $\cdots$\\
\enddata
\tablecomments{The complete table is available in machine-readable form in the online journal; a portion is shown here for guidance on format and content. Owing to its wide format, only the most relevant columns are displayed (see Table \ref{tab:column_description}).}
\end{deluxetable*}
\end{center}
